# Supplementary material for: Discovering Political Topics in Facebook Discussion threads with Graph Contextualization
Source: arXiv:1708.06872 ancillary file (2018-03-24)
Supplement: Supplementary file 1 [file YilinZhang-AOAS-supplementary.pdf]

*Submitted to the Annals of Applied Statistics*

# SUPPLEMENTARY MATERIALS: DISCOVERING POLITICAL TOPICS IN FACEBOOK DISCUSSION THREADS WITH GRAPH CONTEXTUALIZATION

By Yilin Zhang, Marie Poux-Berthe, Chris Wells, Karolina Koc-Michalska, and Karl Rohe

**1. More evidence for the candidate-centered structure.** This section consists of two parts. Section 1.1 provides more details on citizens' attention-ratio. Section 1.2 provides a clustering approach to partition citizens, which returns a very similar partition for citizens to that from the attention-ratio approach. The clustering approach also shows a very clear candidate-centered structure.

1.1. *More details on citizens' attention-ratio.* Figure 1 bins the citizens based on their attention-ratios and citizen-degrees. In each of the nine plots, there appears a sequence of dark hexagons with attention-ratio being one. This indicates that there is a candidate-centered commenting behavior for citizens throughout the network, no matter they actively comment or not: (1) for the citizens who rarely comment (on left), most of them have attention-ratio being one, indicating that they only comment on one candidate-wall; (2) for the citizens who actively comment (on right), there are also quite a few of them only comment on one candidate-wall.

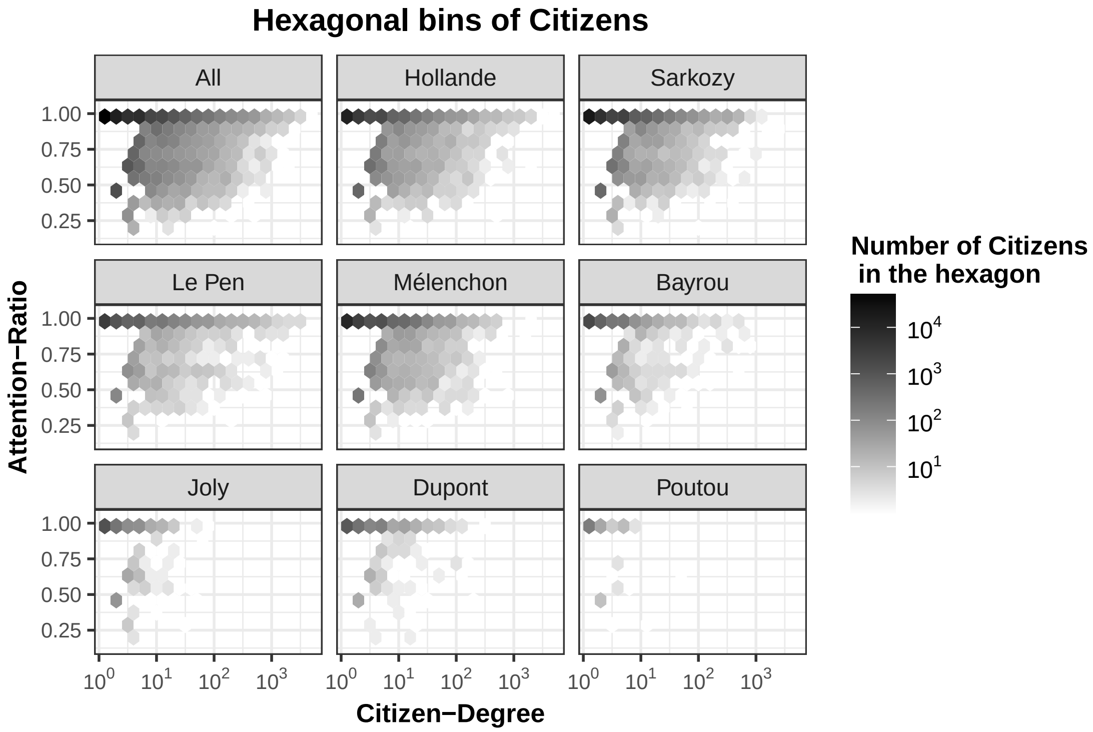


Fig 1. ***Hexagonal Bin Plot for Citizens.*** *The first plot displays the hexagonal bins for all citizens. The rest eight plots are for the eight citizens-clusters which are labeled by the candidates that they focus on.*

1.2. *Clustering approach.* In this section, we provide more evidence for the candidate-centered structure by a clustering approach. We *label each post by which of the eight candidates writes it*, and then partition citizens based on such labels. This is sometimes called stochastic *a priori* blockmodel (Holland et al. (1983), Wasserman and Anderson (1987)). By applying k-means on the rows of matrix $A^{cand} \in \mathbb{R}^{92,226\times 8}$, where for any $i \in \{1,\ldots,N_C\}$ and $j \in \{1,\ldots,N_P\}$,

$$[A^{cand}]_{ij} = \frac{\text{\# of times citizen } i \text{ comments on candidate } j\text{'s wall}}{(\text{\# of comments from citizen } i) \times (\text{\# of posts on candidate } j\text{'s wall})},$$

we get very similar partitions of citizens compared to the attention-ratio approach.[1]

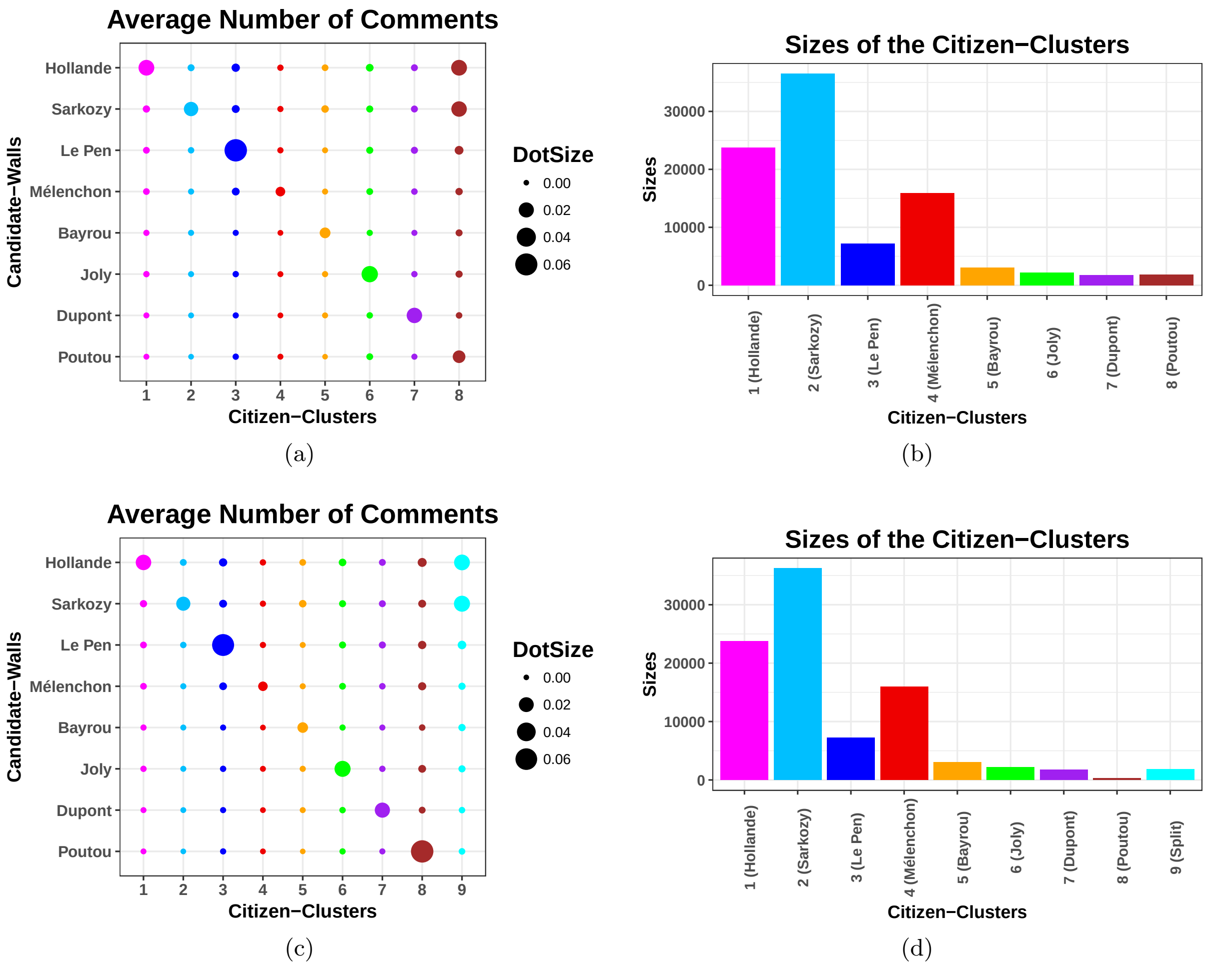


Fig 2. ***Citizen-clusters.*** *Figure (a) and (c) show balloon plots of $\Psi_C$ for the citizen-clusters in the two cases, $K_C = 8$ and $K_C = 9$. Figure (b) and (d) show number of citizens in each cluster when $K_C = 8$ and when $K_C = 9$. In Figure (b) and (d), we label each citizen-cluster by the corresponding candidate . For example, the first citizen-cluster from Figure (a) or (c) is Hollande-centered, so we label it as 1 (Hollande) in Figure (b) or (d).*

When $K_C = 8$, there is a citizen-cluster (the eighth cluster) that splits among three candidates. By increasing the number of citizen-clusters to $K_C = 9$, each candidate has a corresponding citizen-cluster that mainly comment on their posts, while there is a splitting cluster between Hollande and

[1] In either of the two cases, $K_C = 8$ and $K_C = 9$, over 96% of the citizens have the same cluster label with the label from the attention-ratio approach.

Sarkozy. Similar to the attention-approach, the clustering approach also shows a clear candidate-centered structure of the discussion threads.

**2. Choice of $K$ to search for the issue-centered structure.** To search for the issue-centered structure, we choose the number of clusters $K$ by looking at the scree plot of the singular values of the similarity matrix $S$. From Figure 3, there is a large gap after the fourth singular value, so we decide to choose $K = 4$ clusters. By comparing scree plots with different $h$, the increasing of $h$ boosts the first singular value of $S$.

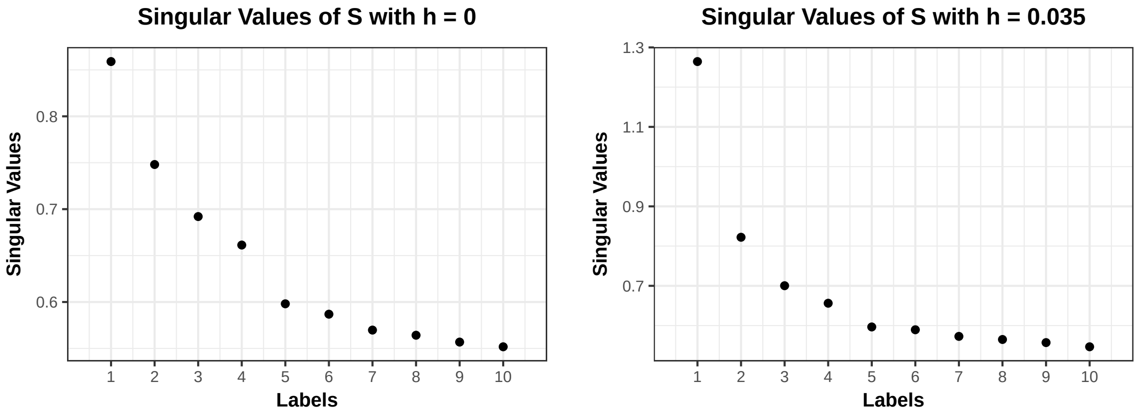


(a) (b)

FIG 3. ***Singular Values of S.***

**3. Different choices for document-term matrices.** In this section, we compare keywords in each cluster using (1) plain (unscaled and unweighted) document-term matrices in Table 1, (2) the scaled document-term matrices (scaled by both rows and columns) in Table 2, and (3) TF-IDF (term frequency-inverse document frequency) document-term matrices in Table 3 (weighted by popularity of words in the documents). For comparison, we set the tunning parameter for `pairGraphText` $h = \infty$.

Table 1 shows the case with plain (unscaled and unweighted) document-term matrices. Compared to the case using scaled document-term matrices in Table 2, more candidates' names appear in the post-cluster 2 in Table 1. Table 3 shows the case with the TF-IDF document-term matrices. More emotional words appear in keywords, but top candidates' names like François Hollande, Nicolas Sarkozy, and Jean-Luc Mélenchon, don't appear in this case.

**4. More simulations for comparison analysis.** In this section, we compare `pairGraphText` with multiple methods, including RTM, CASC, spectral clustering on the graph (which we call L for short), spectral clustering on the text (which we call X for short), and `all-one pairGraphText`.

Simulation settings and choices of parameters in Figure 4 are similar to the settings in Section 6.2.3 in the paper. The only difference is that we simulate 90% of the words as noises. This is due to the fact that most words are irrelevant in real cases, and it helps differ `pairGraphText` (which selects among words) from CASC (which uses all words equally). We simulate these words as noises by adding another block for the words. We define $B^{text} = \begin{pmatrix} 0.1 + sig_t & 0.1 & 0.1 \\ 0.1 & 0.1 + sig_t & 0.1 \end{pmatrix}$, where the text signal $sig_t$ shows the words contain how much block information. Recall that for

Table 1
***Keywords in clusters by `pairGraphText` with plain document-term matrices***

| Citizen-Clusters | |
|---|---|
| Cluster 1 | Nicolas Sarkozy, François Hollande, vote, dwarf, fail, thief, may, president, incompetent, arrogant, liar, captain |
| Cluster 2 | residential, child, descent, aristocrat, clinic, chic, inhabit, pent, land, childhood, employment, discrete |
| Cluster 3 | Koran, angel, Allah, pig, religion, Islam, blue, pig, Arab, Muslim, sister, Lyon, hall, church, mosque, racist |
| Cluster 4 | comrade, Jean-Luc Mélenchon, FDG, troll, front, resistance, revolutionary, liberal, human, moving |

| Post-Clusters | |
|---|---|
| Cluster 1 | arrogant, flamby, goodbye, captain, bravo, debate, incompetent, sir, president, concord, charisma, François Hollande |
| Cluster 2 | modem, centrist, François Bayrou, Nicolas Dupont-Aignan, euros, ecologic, job, resident, ancestry, vineyard, Eva Joly |
| Cluster 3 | Koran, Allah, religion, angel, Islam, Lyon, mosque, Arab, Muslim, sister, pig, religion, Christian, church, racist |
| Cluster 4 | comrade, FDG, resistance, troll, front, Jean-Luc Mélenchon, revolutionary, liberal, human, foul, photos, moving |

Table 2
***Keywords in clusters by `pairGraphText` with scaled document-term matrices***

| Citizen-Clusters | |
|---|---|
| Cluster 1 | François Hollande, Nicolas Sarkozy, fail, president, live, incompetent, May, charisma, arrogant, dwarf, goodbye, liar |
| Cluster 2 | residential, descent, child, clinical, chic, aristocrat, inhabit, land, employment |
| Cluster 3 | Koran, Allah, religion, Islam, angel, pig, pork, Muslim, Arab, racist |
| Cluster 4 | JLM, comrade, resistance, FDG, front, Jean-Luc Mélenchon, liberal, revolutionary, human, capital, ecologic |

| Post-Clusters | |
|---|---|
| Cluster 1 | concord, flamby, sir, president, captain, bravo, charisma, assistantship, arrogant, goodbye, strong, debate, failed, incompetent |
| Cluster 2 | employment, euro, child, residential, pedigree, chic, clinic, pent, inhabit, land |
| Cluster 3 | Koran, religion, Allah, angel, Islam, pig, Muslim, mosque, Arab, Lyon, racist, church |
| Cluster 4 | JLM, comrade, resistance, FDG, troll, Jean-Luc Mélenchon, revolutionary, front, human, struggle, liberal, fight |

Table 3
***Keywords in clusters by `pairGraphText` with TF-IDF document-term matrices***

| Citizen-Clusters | |
|---|---|
| Cluster 1 | zero, abstained, foul, particularly, notch, hype, mischief, suffer, official, patriot, construct, referendum, nation |
| Cluster 2 | angel, Koran, jester, discriminant, hate, dwarf, civilizer, sister, Allah, rag, religion, night, property, Islam |
| Cluster 3 | can, montage, essence, Obama, terrible, central, ambitious, borrowing, aristocrat, pent, cap, chic, radio, hiring, context |
| Cluster 4 | dismissal, damned, illegal, unfair, fraud suppression, leaks, authorized, multiple, reception, September, art, symbol |

| Post-Clusters | |
|---|---|
| Cluster 1 | liar, jester, Koran, dwarf, cheat, thief, euros, multiple, lawyer, religion, angel |
| Cluster 2 | continue, hope, resistance, disgust, fight, battling, modem, struggle, quack, consignment, centrist, proud, can |
| Cluster 3 | concord, modem, Philippe Poutou, passion, centrist, fort, courage, François Bayrou, captain |
| Cluster 4 | Eva Joly, ecologic, south, green, François Bayrou, canal, water, revolutionary, surprised, goodbye |

`pairGraphText`, we set weight $h$ so that the first singular values of the graph Laplacian $L$ and the text assisted part $hC_T$ are equal. Similarly for CASC, we set weight $h$ so that the first singular values of the graph Laplacian $L$ and the text assisted part $hXX^T$ are equal.

From Figure 4, when there are both graph and text signals, all methods can recover block labels with large enough signals. Mis-clustering rate for `pairGraphText` goes to zero fastest compared to all other methods, and mis-clustering rate for L goes to zero at the slowest rate. When there are only

graph signals, L performs the best, followed by `pairGraphText`. Without selecting relevant words, CASC performs worse than `pairGraphText`. When there are only text signals, L and `all-one pairGraphText` fail to recover block lables; X performs the best among all methods, followed by RTM. `pairGraphText` recovers over 90% of the blocks when the signal level is over 1.

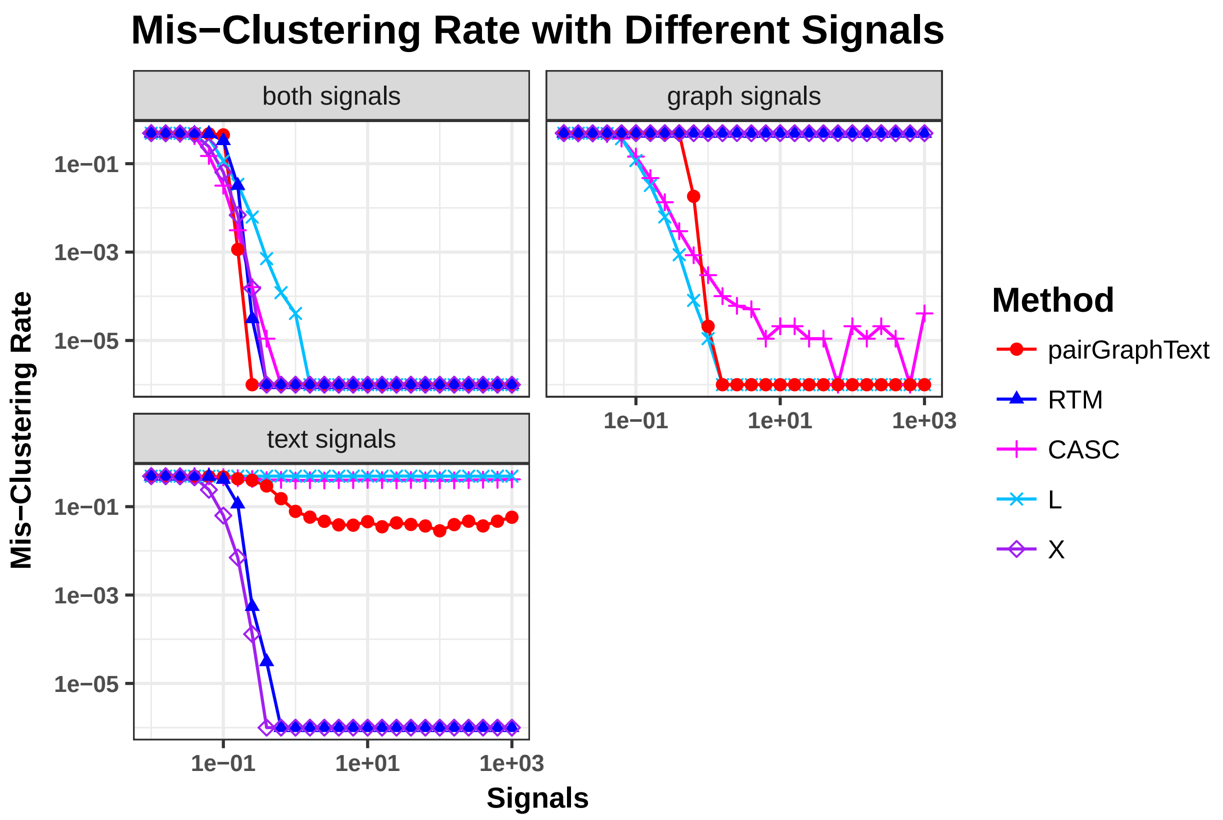


FIG 4. ***Comparison with multiple methods***

Figure 5, 6, and 7 use the same simulation settings as in Figure 4, but their simulation settings generalize to different number of nodes $N \in \{1000, 2000\}$, number of words $M \in \{1000, 2000, 3000\}$, and number of blocks $K \in \{2, 4\}$. With number of blocks $K$ increasing, RTM gets worse. The mis-clustering rate only changes slightly with different values of $N$ and $M$.

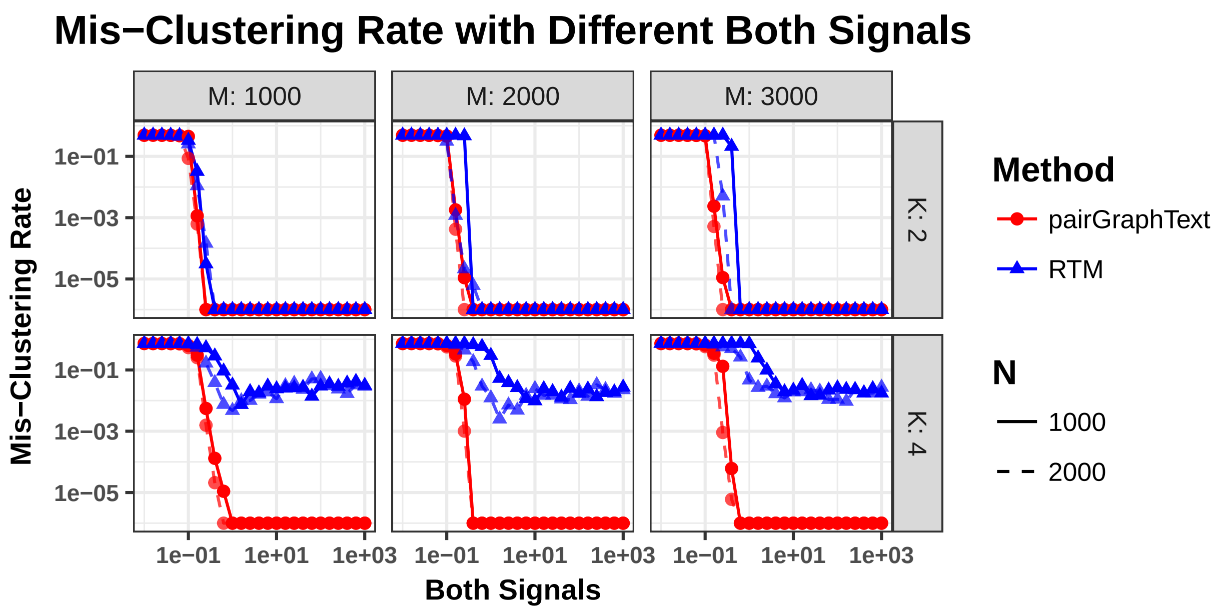


FIG 5. *Compare* `pairGraphText` *and RTM with both graph and text signals*

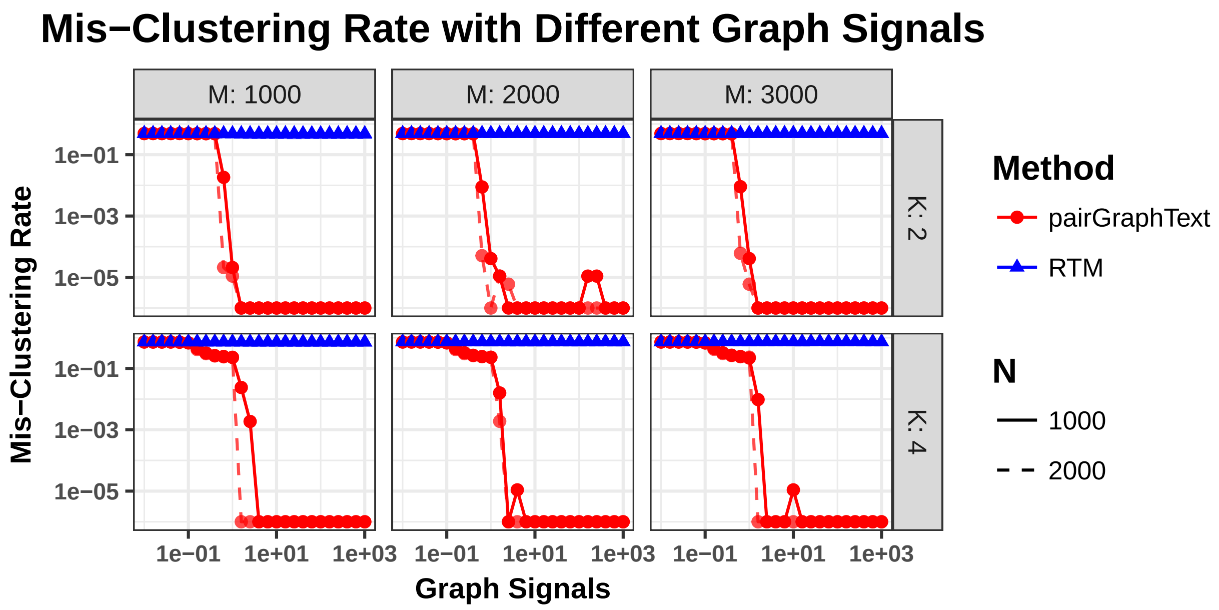


FIG 6. *Compare* `pairGraphText` *and RTM with graph signals*

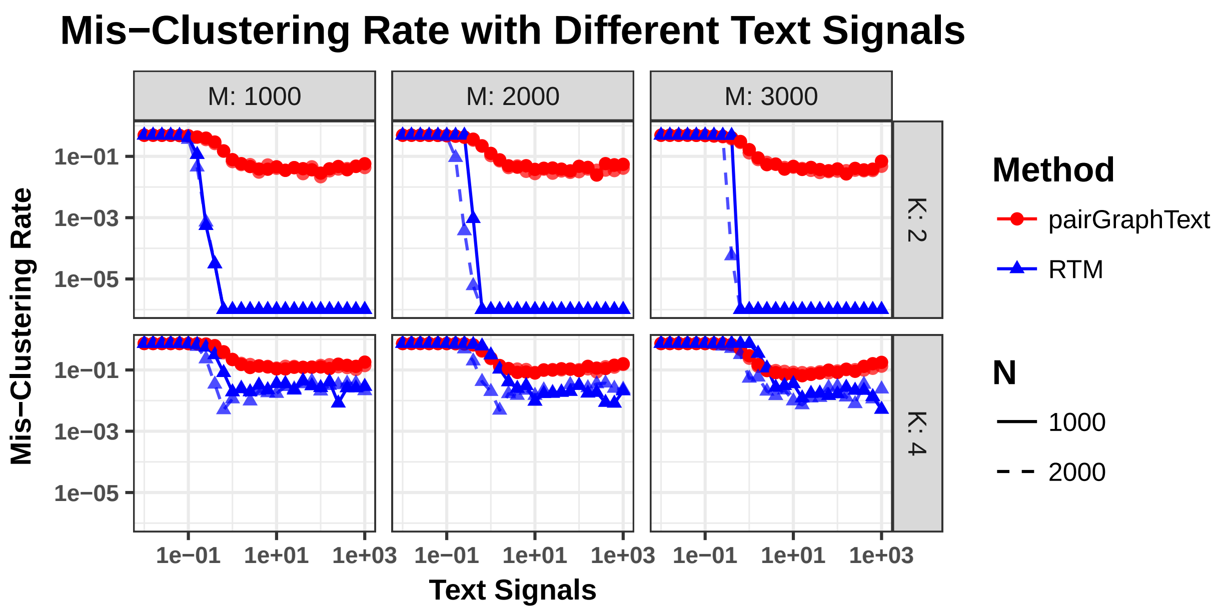


FIG 7. ***Compare pairGraphText and RTM with text signals***

**5. Theoretical justifications for `pairGraphText`.** This section consists of three parts. Section 5.1 shows the equivalence of the population singular spaces and the block membership of nodes. Section 5.2 provides the definition of mis-clustered nodes. Section 5.3 proves Theorem 5.2, the upper bound of the mis-clustering rate.

5.1. *Equivalence of population singular spaces and block membership.* Recall $S$ and $\mathcal{S}$ are the empirical and population similarity matrices for `pairGraphText`, and $U_C$ and $\mathcal{U}_C$($U_P$ and $\mathcal{U}_P$) contain the top $K$ left(right) singular vectors of $S$ and $\mathcal{S}$.

THEOREM 5.1. *Under the NC-ScBM, there exists orthogonal matrices $Q$ and $R$, such that for any $i, j = 1, ..., N$,*

$$\mathcal{U}_C = Z_C(Z_C^T Z_C)^{-1/2} Q \text{ and } [\mathcal{U}_C]_{i\cdot} = [\mathcal{U}_C]_{j\cdot} \iff [Z_C]_{i\cdot} = [Z_C]_{j\cdot},$$
$$\mathcal{U}_P = Z_P(Z_P^T Z_P)^{-1/2} R \text{ and } [\mathcal{U}_P]_{i\cdot} = [\mathcal{U}_P]_{j\cdot} \iff [Z_P]_{i\cdot} = [Z_P]_{j\cdot}.$$

REMARK 5.2. Theorem 5.1 indicates that two citizens (candidate-posts) are in the same block if and only if their corresponding rows of the population singular space $\mathcal{U}_C$ ($\mathcal{U}_P$) are the same. The following proof follows the proof of Lemma 3.1 in Rohe et al. (2011).

PROOF. Under the NC-ScBM, we have $\mathcal{A} = Z_C B Z_P^T$, so the population regularized graph Laplacian $\mathcal{L}$ can be rewritten as

$$\mathcal{L} = \mathcal{D}_C^{-1/2} Z_C B Z_P^T \mathcal{D}_P^{-1/2}.$$

Define

$$B_L = diag(\mathbb{1}^T Z_C B + \tau_c)^{-1/2} B diag(B Z_P^T \mathbb{1} + \tau_p)^{-1/2},$$

where $\mathbb{1}$ is an $N$ vector with all elements being one. Then, we can rewrite $\mathcal{L}$ as

$$\mathcal{L} = Z_C B_L Z_P^T.$$

This follows directly from the following calculation.

Define $z_c(\cdot) : \{1, \ldots, N\} \to \{1, \ldots, K\}$ to represent the partition for citizens, such that for any $i \in \{1, \ldots, N\}$ and $k \in \{1, \ldots, K\}$, $z_c(i) = k$ if citizen $i$ belongs to cluster $k$. Similarly, define $z_p(\cdot)$ to represent the partition for candidate-posts. Denote $n_c(k)$ and $n_p(k)$ as the sizes for the $k$th citizen-cluster and post-cluster.

For any $i, j \in \{1, \ldots, N\}$, element $\mathcal{L}_{ij}$ can be represented by some element of matrix $B_L$ as

$$\begin{aligned}\mathcal{L}_{ij} = \frac{B_{z_c(i)z_p(j)}}{[\mathcal{D}_C]_{ii}^{1/2}[\mathcal{D}_p]_{jj}^{1/2}} =& \frac{B_{z_c(i)z_p(j)}}{[\sum_s n_c(s)B_{z_c(i)s} + \tau_c]^{1/2}[\sum_r n_p(r)B_{rz_p(j)} + \tau_p]^{1/2}} \\ =& \frac{B_{z_c(i)z_p(j)}}{[\mathbb{1}^T Z_C B + \tau_c]_{z_c(i)}^{1/2}[B Z_P^T \mathbb{1} + \tau_p]_{z_p(j)}^{1/2}} \\ =& [B_L]_{z_c(i)z_p(j)}.\end{aligned}$$

Define $\Gamma = B_L + hE_C\mathcal{W}E_P^T$. Then the similarity matrix $\mathcal{S}$ can be rewritten as

$$\mathcal{S} = Z_C \Gamma Z_P^T.$$

Note that the matrix $\Gamma$ has $K$ non-zero singular values for any $h$, with exception of a set of values of measure zero. This is also true for $(Z_C^T Z_C)^{1/2}\Gamma(Z_P^T Z_P)^{1/2}$. So we can apply singular value decomposition:

$$(Z_C^T Z_C)^{1/2}\Gamma(Z_P^T Z_P)^{1/2} = Q\Lambda R^T.$$

Let

$$\mathcal{U}_C = Z_C(Z_C^T Z_C)^{-1/2}Q \text{ and } \mathcal{U}_P = Z_P(Z_P^T Z_P)^{-1/2}R.$$

Clearly, there are $\mathcal{U}_C^T\mathcal{U}_C = I$, $\mathcal{U}_P^T\mathcal{U}_P = I$, and $\mathcal{U}_C\Lambda\mathcal{U}_P^T = \mathcal{L}$. Since

$$det((Z_C^T Z_C)^{-1/2}Q) = det(Z_C^T Z_C)^{-1/2})det(Q) \neq 0,$$

we have

$$[\mathcal{U}_C]_{i\cdot} = [\mathcal{U}_C]_{j\cdot} \iff [Z_C]_{i\cdot} = [Z_C]_{j\cdot} \text{ for any } i, j = 1, \ldots, N.$$

Similarly,

$$[\mathcal{U}_P]_{i\cdot} = [\mathcal{U}_P]_{j\cdot} \iff [Z_P]_{i\cdot} = [Z_P]_{j\cdot} \text{ for any } i, j = 1, \ldots, N.$$

□

5.2. *Definition of mis-clustered.* The definition of mis-clustered is the same as in Rohe et al. (2016). Recall $U_C$ and $\mathcal{U}_C$($U_P$ and $\mathcal{U}_P$) contain the top $K$ left(right) singular vectors of $S$ and $\mathcal{S}$. Denote $[\mu_C]_i$ and $[\nu_C]_i$ as the cluster centroid of citizen $i$ generated by k-means on $U_C$ and $\mathcal{U}_C$. Denote $\mathcal{R}_C$ as the rotation matrice that minimizes $\|U_C\mathcal{R}_C^T - \mathcal{U}_C\|_F$. We define the set of mis-clustered citizens as

$$\mathcal{M}_C = \{i : \text{ there exists } j \neq i, \text{ s.t. } \|[\mu_C]_i\mathcal{R}_C^T - [\nu_C]_i\|_2 > \|[\mu_C]_i\mathcal{R}_C^T - [\nu_C]_j\|_2\}.$$

We similarly define the set of mis-clustered candidate-posts $\mathcal{M}_P$. Theorem 5.2 bounds the mis-clustering rate of citizens and candidate-posts, $\frac{|\mathcal{M}_C|}{N}$ and $\frac{|\mathcal{M}_P|}{N}$.

5.3. *Proof of Theorem 5.2 (upper bound of the mis-clustering rate).* We prove Theorem 5.2 in three steps. Section 5.3.1 and Section 5.3.2 provide the concentration for matrices $W$ and $T_\omega(W)$. Section 5.3.3 provides the concentration for the similarity matrix $S$. Section 5.3.4 provides the concentration for the singular spaces. Then, Theorem 5.2 follows directly with the same technique in the proof of Theorem 3 in Binkiewicz et al. (2017).

5.3.1. *Concentration of* $W$. Recall $\xi = \max(\sigma^2\|L\|_F\sqrt{\ln M}, \sigma^2\|L\|\ln M, \frac{\gamma^2}{\delta}\sqrt{\ln M})$. For any matrix $H$, define $\|H\|_{\max} = \max_{sr}|H|_{sr}$.

LEMMA 5.3. *Suppose $A$, $X$ and $Y$, are the adjacency matrix and the node covariate matrices sampled from the NC-ScBM. Recall $W$ and $\mathcal{W}$ are empirical and population call-response matrices. We have*

$$\|W - \mathcal{W}\|_{\max} = O_P(\xi).$$

PROOF. Define $\mathcal{I} = \mathcal{X}^T L\mathcal{Y}$. From the union bound, the problem breaks into two parts:

$$\|W - \mathcal{W}\|_{\max} \le \|W - \mathcal{I}\|_{\max} + \|\mathcal{I} - \mathcal{W}\|_{\max}.$$

For Part 1, from Hanson-Wright inequality (Theorem 1.1 in Rudelson et al. (2013)) and the union bound, there is

$$\|W - \mathcal{I}\|_{\max} = O_P(\max(\sigma^2\|L\|_F\sqrt{\ln M}, \sigma^2\|L\|\ln M)).$$

For Part 2, we break it into two subparts, Part 2.1 and Part 2.2:

$$\|\mathcal{I} - \mathcal{W}\|_{\max} = \|\mathcal{X}^T(L-\mathcal{L})\mathcal{Y}\|_{\max} \le \|\mathcal{X}^T(L-\mathcal{C})\mathcal{Y}\|_{\max} + \|\mathcal{X}^T(\mathcal{C}-\mathcal{L})\mathcal{Y}\|_{\max},$$

where we define $\mathcal{C} = \mathcal{D}_C^{-1/2} A\mathcal{D}_P^{-1/2}$.

For Part 2.1, recall $\delta = \min(\min_i[\mathcal{D}_C]_{ii}, \min_j[\mathcal{D}_P]_{jj})$,

$$\begin{aligned}
\|\mathcal{X}^T(L-\mathcal{C})\mathcal{Y}\|_{\max} &= \max_{sr}|\sum_{ij}\mathcal{X}_{is}\mathcal{Y}_{jr}\frac{A_{ij}}{\sqrt{[\mathcal{D}_C]_{ii}[\mathcal{D}_P]_{jj}}}(\frac{\sqrt{[\mathcal{D}_C]_{ii}[\mathcal{D}_P]_{jj}}}{\sqrt{[D_C]_{ii}[D_P]_{jj}}} - 1)| \\
&\le \max_{sr}\sum_{ij}|\mathcal{X}_{is}\mathcal{Y}_{jr}|\frac{1}{\delta}\max(|\frac{[\mathcal{D}_C]_{ii}}{[D_C]_{ii}} - 1|, |\frac{[\mathcal{D}_P]_{jj}}{[D_P]_{jj}} - 1|) \\
&= \max_{sr}\sum_{ij}|\mathcal{X}_{is}\mathcal{Y}_{jr}|O_P(\delta^{-3/2}) \\
&= O_P(\frac{\gamma^2}{\delta^{3/2}}).
\end{aligned}$$

The second to last equality is from the following proof. For any $i \in \{1, \ldots, N\}$, from Bernstein inequality,

$$\mathbb{P}(|[D_C]_{ii} - [\mathcal{D}_C]_{ii}| > t) \le 2\exp\{-\frac{\frac{1}{2}t^2}{\sum_j \mathcal{A}_{ij}(1-\mathcal{A}_{ij}) + \frac{1}{3}t}\} \le 2\exp\{-\frac{t^2}{2[\mathcal{D}_C]_{ii} + \frac{2}{3}t}\}.$$

Set $t = \varsigma[\mathcal{D}_C]_{ii}$ for some $0 < \varsigma < \frac{1}{2}$. We get

$$\mathbb{P}(|\frac{[D_C]_{ii}}{[\mathcal{D}_C]_{ii}} - 1| > \varsigma) \le 2\exp\{-\frac{\varsigma^2[\mathcal{D}_C]_{ii}}{2+\frac{2}{3}\varsigma}\} \le 2\exp\{-\frac{\varsigma^2\delta}{2+\frac{2}{3}\varsigma}\}.$$

This implies

$$|\frac{[D_C]_{ii}}{[\mathcal{D}_C]_{ii}} - 1| = O_P(\delta^{-1/2}).$$

So

$$|\frac{[\mathcal{D}_C]_{ii}}{[D_C]_{ii}} - 1| = O_P(\delta^{-1/2}).$$

This is because

$$|\frac{[\mathcal{D}_C]_{ii}}{[D_C]_{ii}} - 1| > \frac{\varsigma}{1-\varsigma} \Rightarrow |\frac{[D_C]_{ii}}{[\mathcal{D}_C]_{ii}} - 1| > \varsigma \text{ for any } 0 < \varsigma < \frac{1}{2}.$$

Similarly,

$$|\frac{[\mathcal{D}_P]_{jj}}{[D_P]_{jj}} - 1| = O_P(\delta^{-1/2}) \text{ for any } j \in \{1, \ldots, N\}.$$

Thus,

$$\max(|\frac{[\mathcal{D}_C]_{ii}}{[D_C]_{ii}} - 1|, |\frac{[\mathcal{D}_P]_{jj}}{[D_P]_{jj}} - 1|) = O_P(\delta^{-1/2}).$$

For Part 2.2, $\|\mathcal{X}^T(\mathcal{C} - \mathcal{L})\mathcal{Y}\|_{\max}$, let's focus on its each element.

$$\begin{aligned}
[\mathcal{X}^T(\mathcal{C} - \mathcal{L})\mathcal{Y}]_{sr} =& \sum_{ij} \mathcal{X}_{is}\mathcal{Y}_{jr} \frac{1}{\sqrt{[\mathcal{D}_C]_{ii}[\mathcal{D}_P]_{jj}}}(A_{ij} - \mathcal{A}_{ij}) \\
=& O_P(\sqrt{\sum_{ij} \mathcal{X}_{is}^2\mathcal{Y}_{jr}^2 \frac{\mathcal{A}_{ij}(1-\mathcal{A}_{ij})}{[\mathcal{D}_C]_{ii}[\mathcal{D}_P]_{jj}}}) \\
=& O_P(\sqrt{\sum_{ij} \mathcal{X}_{is}^2\mathcal{Y}_{jr}^2 \frac{1}{\delta^2}}) \\
=& O_P(\frac{\gamma^2}{\delta}),
\end{aligned}$$

where the second equality is from central limit theorem. From union bound and the fact that the upper tail of standard normal distribution $\psi(x) \leq \frac{\exp\{-x^2/2\}}{x\sqrt{2\pi}}$, we have the upper bound for Part 2.2 as

$$\|\mathcal{X}^T(\mathcal{C} - \mathcal{L})\mathcal{Y}\|_{\max} = O_P(\frac{\gamma^2}{\delta}\sqrt{\ln M}).$$

Thus, we have the upper bound for Part 2 as

$$\|\mathcal{I} - \mathcal{W}\|_{\max} = O_P(\frac{\gamma^2}{\delta^{3/2}} + \frac{\gamma^2}{\delta}\sqrt{\ln M}) = O_P(\frac{\gamma^2}{\delta}\sqrt{\ln M}).$$

Thus,

$$\|W - \mathcal{W}\|_{\max} = O_P(\max(\sigma^2\|L\|_F\sqrt{\ln M}, \sigma^2\|L\|\ln M) + \frac{\gamma^2}{\delta}\sqrt{\ln M}) = O_P(\xi).$$

□

5.3.2. *Concentration of $T_\omega(W)$.* For any matrix $H$, define $\|H\|_{\tilde q} = \max(\max_i \|H_{i\cdot}\|_q, \max_j \|H_{\cdot j}\|_q)$.

LEMMA 5.4. *Suppose $A$, $X$ and $Y$, are the adjacency matrix and the node covariate matrices sampled from the NC-ScBM. Recall $W$ and $\mathcal{W}$ are empirical and population call-response matrices. $T_\omega(W)$ is the empirical call-response matrix after thresholding. For any constant $0 \le q < 1$, if $\omega$ asymptotically dominates $\xi$, i.e. $\xi = o(\omega)$, then*

$$\|T_\omega(W) - \mathcal{W}\| = O_P(\|\mathcal{W}\|_{\tilde q}^q \omega^{1-q} + \xi).$$

*Especially, by setting $q = 0$,*

$$\|T_\omega(W) - \mathcal{W}\| = O_P(\omega).$$

Proof of Lemma 5.4 follows the proof of Theorem 1 in Bickel and Levina (2008).

PROOF. For any matrix $H$, denote $\|H\|_1 = \max_r \sum_s |H_{sr}|$ and $\|H\|_\infty = \max_s \sum_r |H_{sr}|$.

We break the concentration problem into two parts,

$$\|T_\omega(W) - \mathcal{W}\| \le \|T_\omega(W) - T_\omega(\mathcal{W})\| + \|T_\omega(\mathcal{W}) - \mathcal{W}\|.$$

For Part 2, $\|T_\omega(\mathcal{W}) - \mathcal{W}\| \le \|T_\omega(\mathcal{W}) - \mathcal{W}\|_1 \|T_\omega(\mathcal{W}) - \mathcal{W}\|_\infty$. Note that

$$\|T_\omega(\mathcal{W}) - \mathcal{W}\|_1 \le \max_r \sum_s |\mathcal{W}_{sr}| \mathbb{1}\{|\mathcal{W}_{sr}| \le \omega\} \le \omega^{1-q} \|\mathcal{W}\|_{\tilde q}^q.$$

Similar for $\|T_\omega(\mathcal{W}) - \mathcal{W}\|_\infty$. Thus, Part 2

$$\|T_\omega(\mathcal{W}) - \mathcal{W}\| \le \omega^{1-q} \|\mathcal{W}\|_{\tilde q}^q.$$

For Part 1, $\|T_\omega(W) - T_\omega(\mathcal{W})\| \le \|T_\omega(W) - T_\omega(\mathcal{W})\|_1 \|T_\omega(W) - T_\omega(\mathcal{W})\|_\infty$. We bound $\|T_\omega(W) - T_\omega(\mathcal{W})\|_1$ by breaking the concentration into three parts (5.1), (5.2), and (5.3):

$$\|T_\omega(W) - T_\omega(\mathcal{W})\|_1 \le \max_r \sum_s |W_{sr}| \mathbb{1}\{|W_{sr}| > \omega, |\mathcal{W}_{sr}| \le \omega\} \tag{5.1}$$

$$+ \max_r \sum_s |\mathcal{W}_{sr}| \mathbb{1}\{|W_{sr}| \le \omega, |\mathcal{W}_{sr}| > \omega\} \tag{5.2}$$

$$+ \max_r \sum_s |W_{sr} - \mathcal{W}_{sr}| \mathbb{1}\{|W_{sr}| > \omega, |\mathcal{W}_{sr}| > \omega\}. \tag{5.3}$$

For part (5.3),

$$(5.3) \le \max_{sr} |W_{sr} - \mathcal{W}_{sr}| \sum_s |\mathcal{W}_{sr}|^q \omega^{-q} = O_P(\xi \|\mathcal{W}\|_{\tilde q}^q \omega^{-q}) = o_P(\|\mathcal{W}\|_{\tilde q}^q \omega^{1-q}),$$

where the first equation is from Lemma 5.3, and the last equation is from $\xi = o(\omega)$.

For part (5.2),

$$\begin{aligned}(5.2) &\le \max_r \sum_s (|W_{sr} - \mathcal{W}_{sr}| + |W_{sr}|) \mathbb{1}\{|W_{sr}| \le \omega, |\mathcal{W}_{sr}| > \omega\} \\ &\le \max_{sr} |W_{sr} - \mathcal{W}_{sr}| \sum_s \mathbb{1}\{|\mathcal{W}_{sr}| > \omega\} + \max_r \sum_s \omega \mathbb{1}\{|\mathcal{W}_{sr}| > \omega\} \\ &= O_P(\xi \|\mathcal{W}\|_{\tilde q}^q \omega^{-q} + \|\mathcal{W}\|_{\tilde q}^q \omega^{1-q}) \\ &= O_P(\|\mathcal{W}\|_{\tilde q}^q \omega^{1-q}).\end{aligned}$$

For part (5.1), we break the concentration problem into two parts (5.4) and (5.5):

$$(5.1) \leq \max_r \sum_s |W_{sr} - \mathcal{W}_{sr}| \mathbb{1}\{|W_{sr}| > \omega, |\mathcal{W}_{sr}| \leq \omega\} \tag{5.4}$$

$$+ \max_r \sum_s |\mathcal{W}_{sr}| \mathbb{1}\{|W_{sr}| > \omega, |\mathcal{W}_{sr}| \leq \omega\}. \tag{5.5}$$

Part (5.5) is bounded by

$$(5.5) \leq \max_r \sum_s |\mathcal{W}_{sr}| \mathbb{1}\{|\mathcal{W}_{sr}| \leq \omega\} \leq \|\mathcal{W}\|_{\tilde{q}}^q \omega^{1-q}.$$

For part (5.4), take $\beta \in (0, 1)$, the concentration problem is broken into two parts:

$$\begin{aligned}(5.4) \leq &\max_r \sum_s |W_{sr} - \mathcal{W}_{sr}| \mathbb{1}\{|W_{sr}| > \omega, \beta\omega \leq |\mathcal{W}_{sr}| \leq \omega\} + \max_r \sum_s |W_{sr} - \mathcal{W}_{sr}| \mathbb{1}\{|W_{sr}| > \omega, |\mathcal{W}_{sr}| < \beta\omega\} \\ \leq &\max_{sr} |W_{sr} - \mathcal{W}_{sr}| \sum_s \mathbb{1}\{|\mathcal{W}_{sr}| \geq \beta\omega\} + \max_{sr} |W_{sr} - \mathcal{I}_{sr}| \sum_s \mathbb{1}\{|W_{sr} - \mathcal{W}_{sr}| > (1 - \beta)\omega\} \\ \leq &\max_{sr} |W_{sr} - \mathcal{W}_{sr}| \|\mathcal{W}\|_{\tilde{q}}^q \beta^{-q} \omega^{-q} + \max_{sr} |W_{sr} - \mathcal{W}_{sr}| \max_r \sum_s \mathbb{1}\{|W_{sr} - \mathcal{W}_{sr}| > (1 - \beta)\omega\}.\end{aligned}$$

For the latter part, note that

$$\begin{aligned}&P(\max_r \sum_s \mathbb{1}\{|W_{sr} - \mathcal{W}_{sr}| > (1 - \beta)\omega\} > 0) \\ =&P(\max_{sr} |W_{sr} - \mathcal{W}_{sr}| > (1 - \beta)\omega) \\ =&o(1).\end{aligned}$$

The last equation is from Lemma 5.3 and $\xi = o(\omega)$.

So part (5.4) $= O_P(\xi \|\mathcal{W}\|_{\tilde{q}}^q \omega^{-q} + \xi) = O_P(\|\mathcal{W}\|_{\tilde{q}}^q \omega^{1-q} + \xi)$.

Combining part (5.4) and (5.5), part (5.1) $= O_P(\|\mathcal{W}\|_{\tilde{q}}^q \omega^{1-q} + \xi)$.

Combining part (5.1), (5.2) and (5.3), $\|T_\omega(W) - T_\omega(\mathcal{W})\|_1 = O_P(\|\mathcal{W}\|_{\tilde{q}}^q \omega^{1-q} + \xi)$. Similar for $\|T_\omega(W) - T_\omega(\mathcal{W})\|_\infty$. Thus, Part 1

$$\|T_\omega(W) - T_\omega(\mathcal{W})\| = O_P(\|\mathcal{W}\|_{\tilde{q}}^q \omega^{1-q} + \xi).$$

Recall Part 2 $\|T_\omega(\mathcal{W}) - \mathcal{W}\| \leq \omega^{1-q} \|\mathcal{W}\|_{\tilde{q}}^q$. Thus, we have

$$\begin{aligned}\|T_\omega(W) - \mathcal{W}\| \leq &\|T_\omega(W) - T_\omega(\mathcal{W})\| + \|T_\omega(\mathcal{W}) - \mathcal{W}\| \\ =&O_P(\|\mathcal{W}\|_{\tilde{q}}^q \omega^{1-q} + \xi).\end{aligned}$$

□

Recall for any matrix $H$, $sym(H) = \begin{pmatrix} 0 & H \\ H^T & 0 \end{pmatrix}$. With the same procedure with Lemma 5.4, we get the following Corollary 5.5.

Corollary 5.5. *With assumptions in Lemma 5.4,*

$$\|sym(T_\omega(W) - \mathcal{W})\| = O_P(\|\mathcal{W}\|_{\tilde{q}}^q \omega^{1-q} + \xi).$$

*Especially, by setting $q = 0$,*

$$\|sym(T_\omega(W) - \mathcal{W})\| = O_P(\omega).$$

5.3.3. *Concentration of $S$.*

Lemma 5.6. *Recall $a = \sqrt{\frac{3\ln(16N/\epsilon)}{\delta}}$. With assumptions in Theorem 5.2, with probability at least $1-\epsilon$, for large enough $N$,*

$$\|sym(S-\mathcal{S})\| \le c_2 a,$$

*for some constant $c_2$.*

Proof. We break the concentration problem into bounding the three parts:

$$\|sym(S-\mathcal{S})\| \le \|sym(L-\mathcal{L})\| \tag{5.6}$$
$$+h\|sym(X(T_\omega(W)-\mathcal{W})Y^T)\| \tag{5.7}$$
$$+h\|sym(X\mathcal{W}Y^T - \mathcal{X}\mathcal{W}\mathcal{Y}^T)\|. \tag{5.8}$$

From Rohe et al. (2016), with at least probability $1-\frac{\epsilon}{2}$, part (5.6)

$$\|sym(L-\mathcal{L})\| \le 4a.$$

For part (5.8),

$$h\|sym(X\mathcal{W}Y^T - \mathcal{X}\mathcal{W}\mathcal{Y}^T)\| \le 2h\gamma^2\|sym(\mathcal{W})\|.$$

For part (5.7),

$$h\|sym(X(T_\omega(W)-\mathcal{X}L\mathcal{Y})Y^T)\| \le h\gamma^2\|sym(T_\omega(W)-\mathcal{W})\| = O_P(h\gamma^2\omega).$$

The last equation is from Corollary 5.5. So for large enough $N$, with probability at least $1-\frac{\epsilon}{2}$, (5.7) $\le c_3 h\gamma^2\omega$, where $c_3$ is some constant.

Thus, for large enough graph, with probability at least $1-\epsilon$,

$$\|sym(S-\mathcal{S})\| \le 4a + 2h\gamma^2\|\mathcal{W}\|_2 + c_3 h\gamma^2\omega.$$

From condition (3) in Theorem 5.2

$$h \le \min\left(\frac{a}{\gamma^2\|sym(\mathcal{W})\|}, \frac{a}{\gamma^2\omega}\right),$$

we have

$$\|sym(S-\mathcal{S})\| \le 4a + 2a + ca = (6+c_3)a.$$

□

5.3.4. *Concentration of the singular spaces.*

Lemma 5.7. *With assumptions in Theorem 5.2, with probability at least $1-\epsilon$, for large enough $N$, we have*

$$\|U_C - \mathcal{U}_C\mathcal{R}_C\|_F \le \frac{c_4\sqrt{K\ln(16N/\epsilon)}}{\lambda_K\sqrt{\delta}}, \text{ and}$$
$$\|U_P - \mathcal{U}_P\mathcal{R}_P\|_F \le \frac{c_4\sqrt{K\ln(16N/\epsilon)}}{\lambda_K\sqrt{\delta}},$$

*for some constant $c_4$ and some orthogonal matrices $\mathcal{R}_C, \mathcal{R}_P \in \mathbb{R}^{K\times K}$.*

The proof of Lemma 5.7 is almost the same as the proof of Theorem 2 in Binkiewicz et al. (2017).

Theorem 5.2 follows directly from Lemma 5.7 with the same technique in the proof of Theorem 3 in Binkiewicz et al. (2017).

## References.


Bickel, P. J. and Levina, E. (2008). Covariance regularization by thresholding. *The Annals of Statistics*, pages 2577–2604. 5.3.2

Binkiewicz, N., Vogelstein, J., and Rohe, K. (2017). Covariate-assisted spectral clustering. *Biometrika*, 104(2):361–377. 5.3, 5.3.4

Holland, P. W., Laskey, K. B., and Leinhardt, S. (1983). Stochastic blockmodels: First steps. *Social networks*, 5(2):109–137. 1.2

Rohe, K., Chatterjee, S., and Yu, B. (2011). Spectral clustering and the high-dimensional stochastic blockmodel. *The Annals of Statistics*, pages 1878–1915. 5.2

Rohe, K., Qin, T., and Yu, B. (2016). Co-clustering directed graphs to discover asymmetries and directional communities. *Proceedings of the National Academy of Sciences*, 113(45):12679–12684. 5.2, 5.3.3

Rudelson, M., Vershynin, R., et al. (2013). Hanson-wright inequality and sub-gaussian concentration. *Electron. Commun. Probab*, 18(82):1–9. 5.3.1

Wasserman, S. and Anderson, C. (1987). Stochastic a posteriori blockmodels: Construction and assessment. *Social Networks*, 9(1):1–36. 1.2
